# Supplementary material for: GeoAvatar: Adaptive Geometrical Gaussian Splatting for 3D Head Avatar
Source: arXiv:2507.18155 source file (2025-07-24)
Supplement: Supplementary file 1 [file appendix_application.pdf]

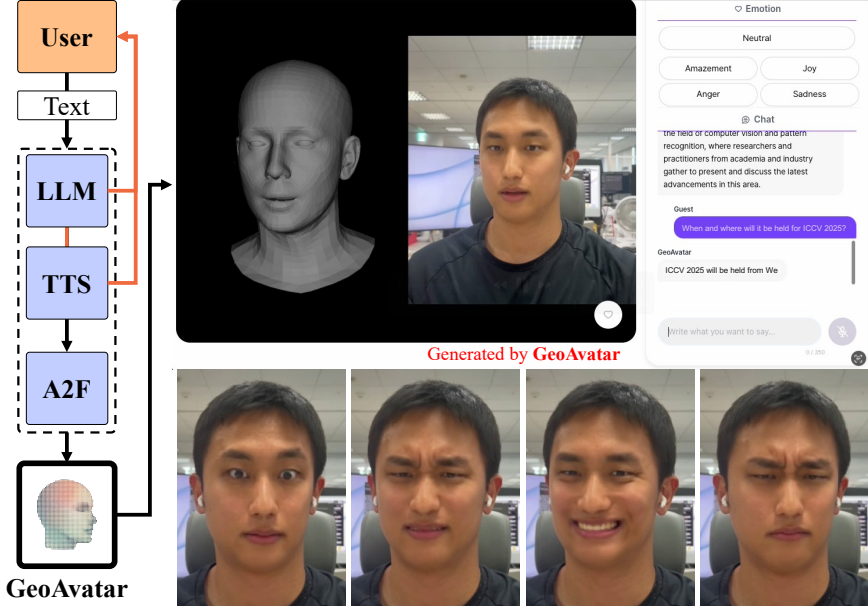

(a) Application #1: Interactable Digital Human

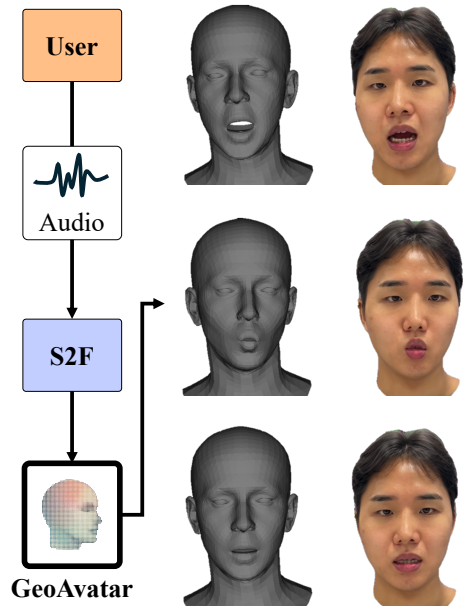

(b) Application #2: Virtual Presentation
