# Supplementary material for: GeoAvatar: Adaptive Geometrical Gaussian Splatting for 3D Head Avatar
Source: arXiv:2507.18155 source file (2025-07-24)

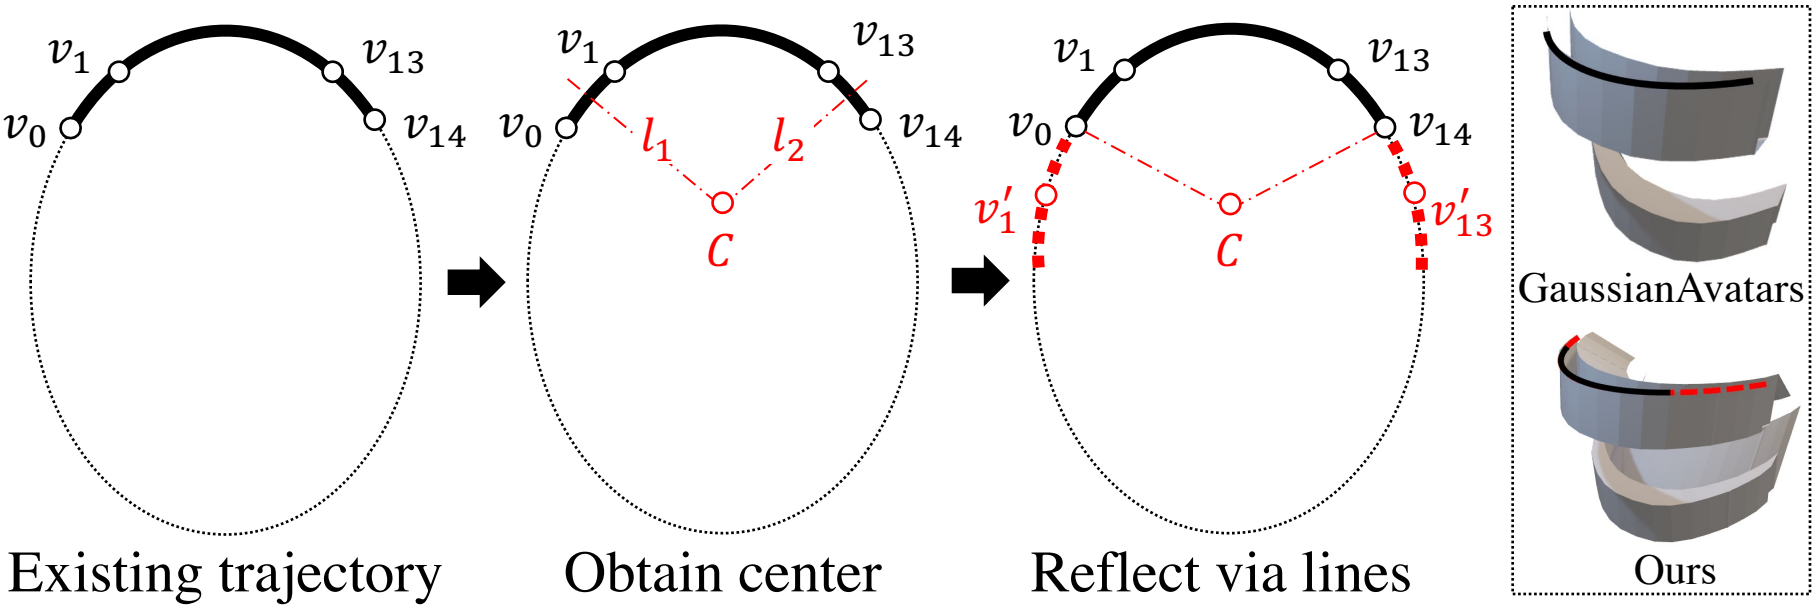

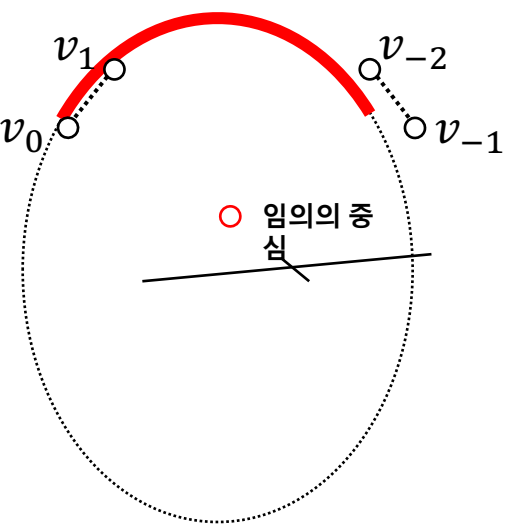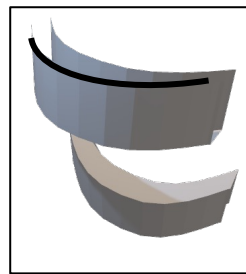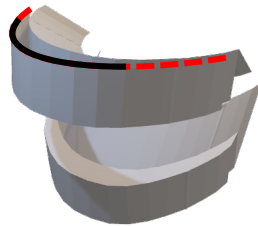

Supplement: Supplementary file 2 [file appendix_teeth.pdf]
